# Supplementary material for: FlipOut: Uncovering Redundant Weights via Sign Flipping
Source: arXiv:2009.02594 source file (2020-09-05)
Supplement: Supplementary file 1 [file appendix.tex]

\section*{\huge{Supplementary Material}}

\section{Dataset preprocessing and models}
\label{appendix:datasets_and_models}
\subsection{Experiments on CIFAR-10}
CIFAR-10 (\cite{cifar10}, \cite{cifar10_link}) is an image classification dataset, consisting of 60000 images of size $32\times32\times3$, each belonging to one of ten mutually exclusive classes. Each class has 5000 training images and 1000 testing images. We have split the dataset into 50000 images for training and 10000 for testing. Data augmentation was applied to the training set, utilizing padding, random cropping and random horizontal flipping. For both the training and test sets, the color channels of the images were normalized to the means and standard deviation of each color channel as computed on the training set. The original dataset can be downloaded from 

The implementation of the ResNet-18 (\cite{resnet}) and VGG-19 (\cite{vgg}) models as well as the hyperparameters used for all experiments in our work are directly taken from \cite{pytorch_cifar_10}. 

\subsection{Experiments on ImageNette}
According to the official repository published by \cite{imagenette_dataset}, "Imagenette is a subset of 10 easily classified classes from Imagenet", where Imagenet is a large scale object classification dataset introduced by \cite{imagenet_cvpr09}. Imagenette contains approximately 13400 images of various sizes, of which $9469$ in the training set and $3925$ in the test set, in an approximately $70-30$ split. All images have been resized to $224 \times 224 \times 3$ pixels. For grayscale images, two duplicates of the single color channel have been generated and stacked on top of the original image, simulating an RGB format. Data augmentation and normalization were performed in the same manner as for the CIFAR-10 dataset. For this dataset, we use DenseNet121 , as presented in \cite{densenet} and implemented in the Pytorch Torchvision framework (\cite{pytorch}, \cite{torchvision_link}).

\section{Experimental setup}
\label{appendix:experimental_setup}
In this section we go into more detail regarding the setup of our experiments and motivate our choices.
\subsection{Batch normalization parameters should not be pruned}
Batch normalization layers (\cite{batchnorm}) are used in many neural network architectures in order to normalize the inputs to each layer, thus preserving gradient flow and allowing for better training. Given the previous layer's activations $x=\{x_{1\dots m}\}$ over a mini-batch $\mathcal{B}$ of $m$ samples, the batch normalization first computes the empirical mean $\mu_\mathcal{B}$ and variance $\sigma_\mathcal{B}^2$ of the mini-batch activations. The outputs $y=\{y_{1\dots m}\}$ are, then:
\begin{equation*}
\begin{split}
\hat{x}_i \leftarrow \frac{x_i - \mu_\mathcal{B}}{\sqrt{\sigma_\mathcal{B}^2 + \epsilon}} \\
y_i \leftarrow \gamma \hat{x}_i + \beta
\end{split}
\end{equation*}
The learnable parameters, $\gamma$ and $\beta$ are used to scale and shift the distribution once the inputs are normalized. Pruning these parameters can cause unintended consequences. For instance, let us consider the batch normalization output $y_i$ for a single training instance from a mini-batch. For a linear layer of $n$ neurons, $y_i$ is a vector of size $n$; similarly, for a convolutional layer of $n$ filters, $y_i$ will also be of size $n$. If we have $\gamma_k=0$, i.e. the $k$-th dimension of $\gamma$ has been pruned, we then have $y_{ik}=\beta_k$ for all samples in the mini-batch, which can impede training. Moreover, if both $\gamma_k$ and $\beta_k$ are equal to $0$, we have $y_{ik}=0$. Since the input to the next layer is $\zeta(y)$, for an activation function $\zeta$ with $\zeta(0)=0$, such as the commonly used ReLU (\cite{relu}) or sigmoid activations, the input to the next layer after batch normalization will also be $0$. This is equivalent to pruning all weights that contributed to generating that output activation, i.e. all weights inbound to a neuron or the weights that form a filter, since they now no longer contribute to the network's output. In doing so, one could effectively prune more weights than intended, which can impact accuracy. To avoid this, we have chosen not to prune these parameters. Another important observation is that at inference time, batch normalization only uses population statistics, and is independent of $\beta$ and $\gamma$:
\begin{equation*}
    y = \hat{x} = \frac{x-\E[x]}{\sqrt{Var[x]+\epsilon}}
\end{equation*}
Therefore, pruning them offers no benefit once training is done.
During our experiments, batch normalization parameters have not been pruned for any of the methods tested.

\subsection{Global pruning}
As \cite{lth} have noted, for deep networks, where the number of parameters per layer can vary significantly, pruning layers separately at the same rate can cause the smaller layers to become bottlenecks, impacting accuracy. In order to alleviate this problem, the authors suggest using global pruning, that is, when selecting the weights to be removed, they are ranked collectively across all layers. We apply this strategy for FlipOut as well as for the pruning methods we compare to.

\section{Choosing the hyperparameters for FlipOut}
\label{appendix:choosing_hyperparameters}
FlipOut uses a saliency criterion for each weight based on its magnitude and the number of sign flips that it has undergone throughout training. To reiterate, at time step $t$, the saliency $\tau_j^t$ of a weight $\theta_j^t$ is computed as:

\begin{subequations}
\begin{align*}
    \tau_j^t &= \frac{|\theta_j^t|^{p}}{\text{flips}_j^t} \\
    \text{flips}_j^t &= \sum_{i=0}^{t-1} [\text{sgn}(\theta_j^i) \neq \text{sgn}(\theta_j^{i+1})]
\end{align*}
\end{subequations}

The hyperparameter $p$ weights the importance of the magnitude relative to the number of sign flips when making a pruning decision.
At the same time, to increase the reliability of the signal, gradient noise is added at each step of SGD, scaled by the $L_2$ norm of each layer. At layer $l$ of dimensionality $d_l$, its gradient is modified as:

\begin{align*}
    \bm{\hat{g}}^{t,l} &\leftarrow \bm{g}^{t,l} + \lambda \bm{\epsilon} \\
    \bm{\epsilon} &\sim \mathcal{N}(0, \sigma_{t,l}^2) \\
    \sigma_{t,l}^2 &= \frac{\| \bm{\theta}^{t,l}\|_2^2}{d_l} 
\end{align*}

Here, $\lambda$ controls how much noise is added.

We have experimented with different values of the two hyperparameters, $p$ and $\lambda$ and found that $p=2$ and $\lambda=1$ offer consistent, strong results for all networks tested. In the following paragraphs, we detail the procedure used in determining these values.

For $\lambda$, we have ran all networks at $15$ different values, ranging from $0.75$ to $1.5$ in increments of $0.05$. The value of $p=2$ was used. The networks were evaluated on a validation set, created by removing a subset of samples from the training set. The size of the validation set was $10000$ for CIFAR10 and $2000$ for Imagenette. For our subsequent experiments, (Sections \ref{section:results} and \ref{section:noise_ablation}), the networks have been trained on both the training and validation sets.  As a metric, we have used the accuracy of the networks at the end of training for the sparsity levels of $93.75\%$ and $99.9\%$. We provide the values for these runs in Table \ref{table:lambda_gridsearch}. Notice that the differences are almost negligible at $93.75\%$ sparsity. For the larger sparsity level the disparity increases, although the default value still remains within $2$ percentage points of the optimum value for all networks considered. The largest gap can be seen for ResNet and DenseNet121, at approximately $1.7$ and $1.5$ percentage points, respectively. Since there are only two out of six cases in which optimizing $\lambda$ has helped beyond a negligible amount, we have used the value of $1$ for this hyperparameter throughout our experiments.

\begin{table}
  \vspace{10pt}
  \caption{Accuracies when using the best value of $\lambda$ discovered by grid search separately on two levels of sparsity and the default value of $\lambda=1$. For DenseNet-121 at $93.75\%$ sparsity, the default value was also the optimum.}
  \vspace{10pt}
  \label{table:lambda_gridsearch}
  \centering
  \begin{tabular}{lllll}
    \toprule
    & \multicolumn{2}{c}{Acc. at sparsity $93.75\%$} & \multicolumn{2}{c}{Acc. at sparsity $99.9\%$} \\
    \cmidrule(r){2-3}
    \cmidrule(r){4-5}
    Model & $\lambda^*$ & $\lambda=1$ & $\lambda^*$ & $\lambda=1$ \\
    \midrule
    ResNet18 & 94.58 & 94.56 & 83.75 & 82.07 \\
    VGG19 & 93.07 & 92.96 & 87.72 & 87.24 \\
    DenseNet121 & 89.75 & 89.75 & 73.5 & 72.05 \\
    \bottomrule
  \end{tabular}
\end{table}

We repeat these experiments for $p$ on four values, $p \in \{0, \frac{1}{2}, 1, 2\}$. As can be seen in Table \ref{table:p_gridsearch}, the value of $p=2$ consistently outperforms all other tested values. 

We recommend the two hyperparameter values found through these experiments to practitioners that wish to extend FlipOut to new use-cases.

\begin{table}
  \vspace{10pt}
  \caption{Table of results for different values of $p$ at two levels of sparsity.}
  \vspace{10pt}
  \label{table:p_gridsearch}
  \centering
  \begin{tabular}{lllllllll}
    \toprule
    & \multicolumn{4}{c}{Acc. at sparsity $93.75\%$} & \multicolumn{4}{c}{Acc. at sparsity $99.9\%$} \\
    \cmidrule(r){2-5}
    \cmidrule(r){6-9}
    Model & $p=0$ & $p=\frac{1}{2}$ & $p=1$ & $p=2$ & $p=0$ & $p=\frac{1}{2}$ & $p=1$ & $p=2$ \\
    \midrule
    ResNet18 & 93.71 & 88.39 & 94.18 & \textbf{94.26} & 72.69 & 77.08 & 79.83 & \textbf{82.07} \\
    VGG19 & 91.68 & 82.44 & 92.56 & \textbf{92.96} & 81.48 & 80.69 & 86.01 & \textbf{87.24} \\
    DenseNet121 & 10.35 & 77.40 & 88.9 & \textbf{89.75} & 10.35 & 10.35 & 70.85 & \textbf{72.05} \\
    \bottomrule
  \end{tabular}
\end{table}

\section{Ablation study on the noise}
\label{appendix:noise_ablation_figure}
We provide the results from our experiments in Section \ref{section:noise_ablation}, which can be seen in Fig. \ref{fig:noise_ablation}. 

\begin{figure}[t]
  \centering
  \subfloat[ResNet18 on CIFAR10]{\label{fig:noise_ablation_rn18}\includegraphics[width=60mm]{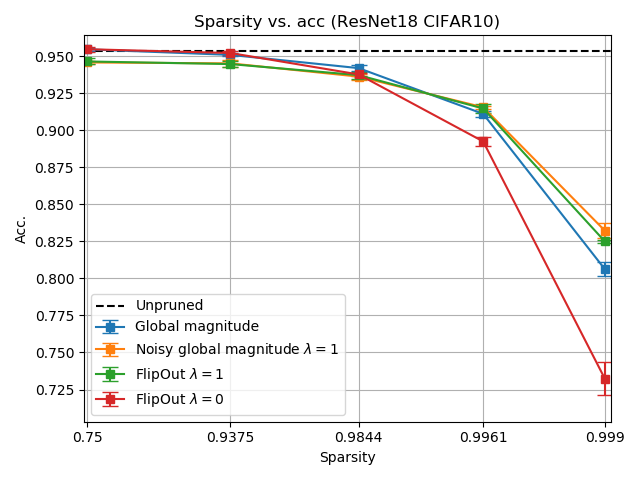}}
  \subfloat[VGG19 on CIFAR10]{\label{fig:noise_ablation_vgg19}\includegraphics[width=60mm]{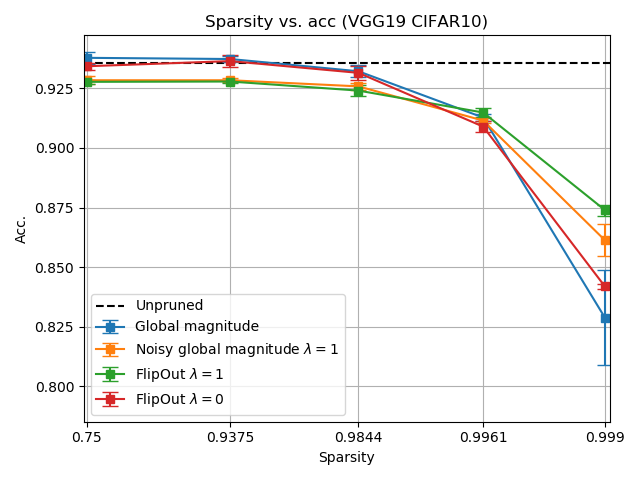}}
  \\
  \subfloat[DenseNet121 on Imagenette]{\label{fig:noise_ablation_dn121}\includegraphics[width=60mm]{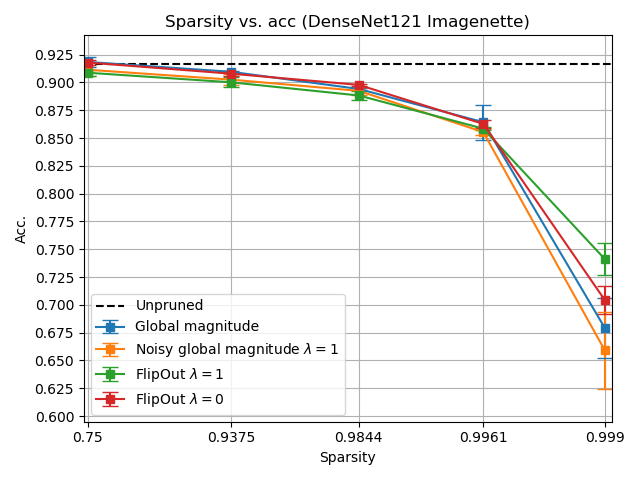}}
  \vspace{10pt}
  \caption{Results of the ablation study on the noise. The accuracy of the unpruned network is illustrated as a horizontal dotted line. Global magnitude without adding noise is also shown for comparison. Each point is the average over 3 different seeds; error bars indicate standard deviation.}
  \label{fig:noise_ablation}
\end{figure}
